# Supplementary material for: Ftklipse - Design and Implementation of an Extendable Computer Forensics Environment: Software Requirements Specification Document
Source: arXiv:0906.2446 source file (2009-07-27)
Supplement: Supplementary file 1 [file appendix.tex]

\appendix

%\chapter{Something Appendiceful}

%\chapter{ChangeLog}

%\vspace{15pt}
%\hrule
%{\scriptsize \input{ChangLog}}
%\hrule
%\vspace{15pt}

% EOF
